# Supplementary material for: Absolute-Unified Multi-Class Anomaly Detection via Class-Agnostic Distribution Alignment
Source: arXiv:2404.00724 source file (2024-04-16)
Supplement: Supplementary file 1 [file supp.tex]

\title{Appendix of Absolute-Unified Multi-Class Anomaly Detection via Class-Agnostic Distribution Alignment}
